# Supplementary material for: Soteria: A Provably Compliant User Right Manager Using a Novel Two-Layer Blockchain Technology
Source: arXiv:2003.10128 source file (2020-03-24)
Supplement: Supplementary file 1 [file Appendix-Alison.tex]

\section{Appendix}
\label{sec:app}
\subsection{API Definition}

%\begin{center}
\begin{table*}[h!]
\small
\centering
% Create New Directory
\begin{tabular}{ | m{2.5cm} || m{11.5cm} | } 
 \hline
 \multicolumn{2}{|c|}{\em Create New directory} \\
 \hline
 Description & Create a new directory to be used by a DDS \\
 \hline
 Method \& URL & POST https://dxdl.deepq.com:5000/directory/new/ \\
 \hline
 Parameters & (None) \\ 
 \hline
 Success Response & code=200, message="A new directory is created and deployed.", txHash=({\em transaction hash}), directoryID=({\em directory address}),  \\
 \hline
 Error Response & code=400, error=({\em error message}) \\
 \hline
\end{tabular}

%\hfill \break

% User Registration
\begin{tabular}{ | m{2.5cm} || m{11.5cm} | } 
 \hline
 \multicolumn{2}{|c|}{\em User Registration} \\
 \hline
 Description & Register a user (provider or consumer) \\
 \hline
 Method \& URL & POST https://dxdl.deepq.com:5000/user/register/ \\
 \hline
 Parameters & Required: directoryID=[String], userType=[String] ("provider" or "consumer"), userID=[String], password=[String] \\ 
 \hline
 Success Response & code=200, message="Register user successfully." \\
 \hline
 Error Response & code=400, error=({\em error message}) \\
 \hline
\end{tabular}

%\hfill \break

% Data Entry Creation
\begin{tabular}{ | m{2.5cm} || m{11.5cm} | } 
 \hline
 \multicolumn{2}{|c|}{\em Data Entry Creation} \\
 \hline
 Description & Create a new data entry by a provider \\
 \hline
 Method \& URL & POST https://dxdl.deepq.com:5000/entry/create/ \\
 \hline
 Parameters & Required: directoryID=[String], userID=[String], password=[String], offerPrice=[Uint], dueDate=[Uint], dataCertificate=[String], dataOwner=[String], dataDescription=[String], dataAccessPath=[String] \\
 \hline
 Success Response & code=200, message="DEC transaction is written.", txHash=({\em transaction hash}) \\
 \hline
 Error Response & code=400, error=({\em error message}) \\
 \hline
\end{tabular}

%\hfill \break

% EAS Deployment
\begin{tabular}{ | m{2.5cm} || m{11.5cm} | } 
 \hline
 \multicolumn{2}{|c|}{\em EAS Deployment} \\
 \hline
 Description & Deploy a new EAS for a provider and a consumer by the DDS \\
 \hline
 Method \& URL & POST https://dxdl.deepq.com:5000/eas/deploy/ \\
 \hline
 Parameters & Required: directoryID=[String], userID=[String], dataCertificate=[String], expirationDate=[Uint], providerAgreement=[String], consumerAgreement=[String] \\
 \hline
 Success Response & code=200, message="EASD transaction is written.") \\
 \hline
 Error Response & code=400, error=({\em error message}) \\
 \hline
\end{tabular}

%\hfill \break

% EAS Revocation
\begin{tabular}{ | m{2.5cm} || m{11.5cm} | }  
 \hline
 \multicolumn{2}{|c|}{\em EAS Revocation} \\
 \hline
 Description & Revoke an EAS by a user (provider or consumer) \\
 \hline
 Method \& URL & POST https://dxdl.deepq.com:5000/eas/revoke/ \\
 \hline
 Parameters & Required: directoryID=[String], userType=[String] ("provider" or "consumer"), userID=[String], password=[String], EASID=[String] \\
 \hline
 Success Response & code=200, message="EASR transaction ({\em provider or consumer}) is written.", txHash=({\em transaction hash}) \\
 \hline
 Error Response & code=400, error=({\em error message}) \\
 \hline
\end{tabular}

%\hfill \break

% Data Entry Count
\begin{tabular}{ | m{2.5cm} || m{11.5cm} | }  
 \hline
 \multicolumn{2}{|c|}{\em Data Entry Count} \\
 \hline
 Description & Retrieve data entry count in a directory \\
 \hline
 Method \& URL & GET https://dxdl.deepq.com:5000/entry/count/ \\
 \hline
 Parameters & Required: directoryID=[String] \\
 \hline
 Success Response & code=200, message="Data entry count is retrieved.", entryCount=({\em the number of data entry in the directory}) \\
 \hline
 Error Response & code=400, error=({\em error message}) \\
 \hline
\end{tabular}

%\hfill \break

% Data Entry Retrieval by Index
\begin{tabular}{ | m{2.5cm} || m{11.5cm} | }  
 \hline
 \multicolumn{2}{|c|}{\em Data Entry Retrieval by Index} \\
 \hline
 Description & Retrieve a data entry in a directory by entry index \\
 \hline
 Method \& URL & GET https://dxdl.deepq.com:5000/entry/index/ \\
 \hline
 Parameters & Required: directoryID=[String], index=[Uint] \\
 \hline
 Success Response & code=200, message="Data entry is retrieved by index.", providerID=({\em provider ID}),  offerPrice=({\em data offer price}), dueDate=({\em entry due date}), dataCertificate=({\em data certificate}), dataOwner=({\em data owner code}), dataDescription=({\em data description}), dataAccessPath=({\em data access path}), isSearched=({\em true or false, indicating whether the entry can be displayed}), commitTime=({\em timestamp of data entry creation}) \\
 \hline
 Error Response & code=400, error=({\em error message}) \\
 \hline
\end{tabular}

%\hfill \break

% Data Entry Retrieval by Data Certificate
\begin{tabular}{ | m{2.5cm} || m{11.5cm} | }  
 \hline
 \multicolumn{2}{|c|}{\em Data Entry Retrieval by Data Certificate} \\
 \hline
 Description & Retrieve a data entry in a directory by data certificate \\
 \hline
 Method \& URL & GET https://dxdl.deepq.com:5000/entry/dctf/ \\
 \hline
 Parameters & Required: directoryID=[String], dataCertificate=[String] \\
 \hline
 Success Response & code=200, message="Data entry is retrieved by data certificate.", providerID=({\em provider ID}),  offerPrice=({\em data offer price}), dueDate=({\em entry due date}), dataCertificate=({\em data certificate}), dataOwner=({\em data owner code}), dataDescription=({\em data description}), dataAccessPath=({\em data access path}), isSearched=({\em true or false, indicating the entry can be displayed or not}), commitTime=({\em timestamp of data entry creation}) \\
 \hline
 Error Response & code=400, error=({\em error message}) \\
 \hline
\end{tabular}

%\hfill \break

% EAS Retrieval
\begin{tabular}{ | m{2.5cm} || m{11.5cm} | }  
 \hline
 \multicolumn{2}{|c|}{\em EAS Retrieval} \\
 \hline
 Description & Retrieve EAS information by an EAS ID \\
 \hline
 Method \& URL & GET https://dxdl.deepq.com:5000/eas/sid/ \\
 \hline
 Parameters & Required: EASID=[String] \\
 \hline
 Success Response & code=200, message="EAS is retrieved by EASID.", providerID=({\em provider ID}),  offerPrice=({\em data offer price}), dataCertificate=({\em data certificate}), expirationDate=({\em data expiration date}), dataOwner=({\em data owner code}), dataDescription=({\em data description}), dataAccessPath=({\em data access path}), consumerID=({\em consumer ID}), deploymentTime=({\em timestamp of EAS deployment}), providerAgreement=({\em provider agreement}), consumerAgreement=({\em consumer agreement}), isValid=({\em true or false, indicating the EAS is valid or revoked}) \\
 \hline
 Error Response & code=400, error=({\em error message}) \\
 \hline
\end{tabular}

%\hfill \break

%\end{center}
\end{table*}

\subsection{Project}

Implementing MedXchange using the APIs documented in 7.1.

The goal of this term project is to build a data buying and selling platform, Sellers can upload  metadata of data items, and buyers can search for data they want to purchase, negotiate an 
executable agreement script (EAS), and then invoke the validated EAS to access the data. 

We will provide the ledger component (DTL).  This project does not require you to implement
the auditing service (ATS). You are required to implement only the data directory service (DDS).

The following functions are required to be implemented for DDS: 
\begin{itemize}
\item DDSs implemented by students should create their own directory to save data information,
\item Buyers and sellers can register accounts on DDS,
\item A seller can upload data information to the directory created by DDS,
\item A buyer can search data on DDS, which consists of all sellers' data information,
\item A buyer can browse the data information of all available data (not the deleted ones),
\item When an EAS has been established between a buyer and a seller, the EAS is deployed by DDS on
Ethereum, 
\item A buyer or a seller can browse all EAS' that he/she has deployed or revoked,
\item An EAS is invoked by the buyer to access the data,
and 
\item Either a buyer or a seller can revoke an EAS.
\end{itemize}

{\bf Extra bonus credit}: implement a {\color{red} data certificate} service.
